# Supplementary material for: Does DINOv3 Set a New Medical Vision Standard? Benchmarking 2D and 3D Classification, Segmentation, and Registration
Source: arXiv:2509.06467 source file (2026-01-17)
Supplement: Supplementary file 1 [file appendix.tex]

% \newpage
\appendix
